# Supplementary material for: Characterization of the Imbalance Problem on Complete Bipartite Graphs
Source: arXiv:2111.00154 source file (2021-11-20)
Supplement: Supplementary file 1 [file appendix.tex]

\section{Appendix - Figures}
\subsection{Introduction}
\begin{figure}[H]
	\centering
	\includegraphics[width=0.70795\linewidth]{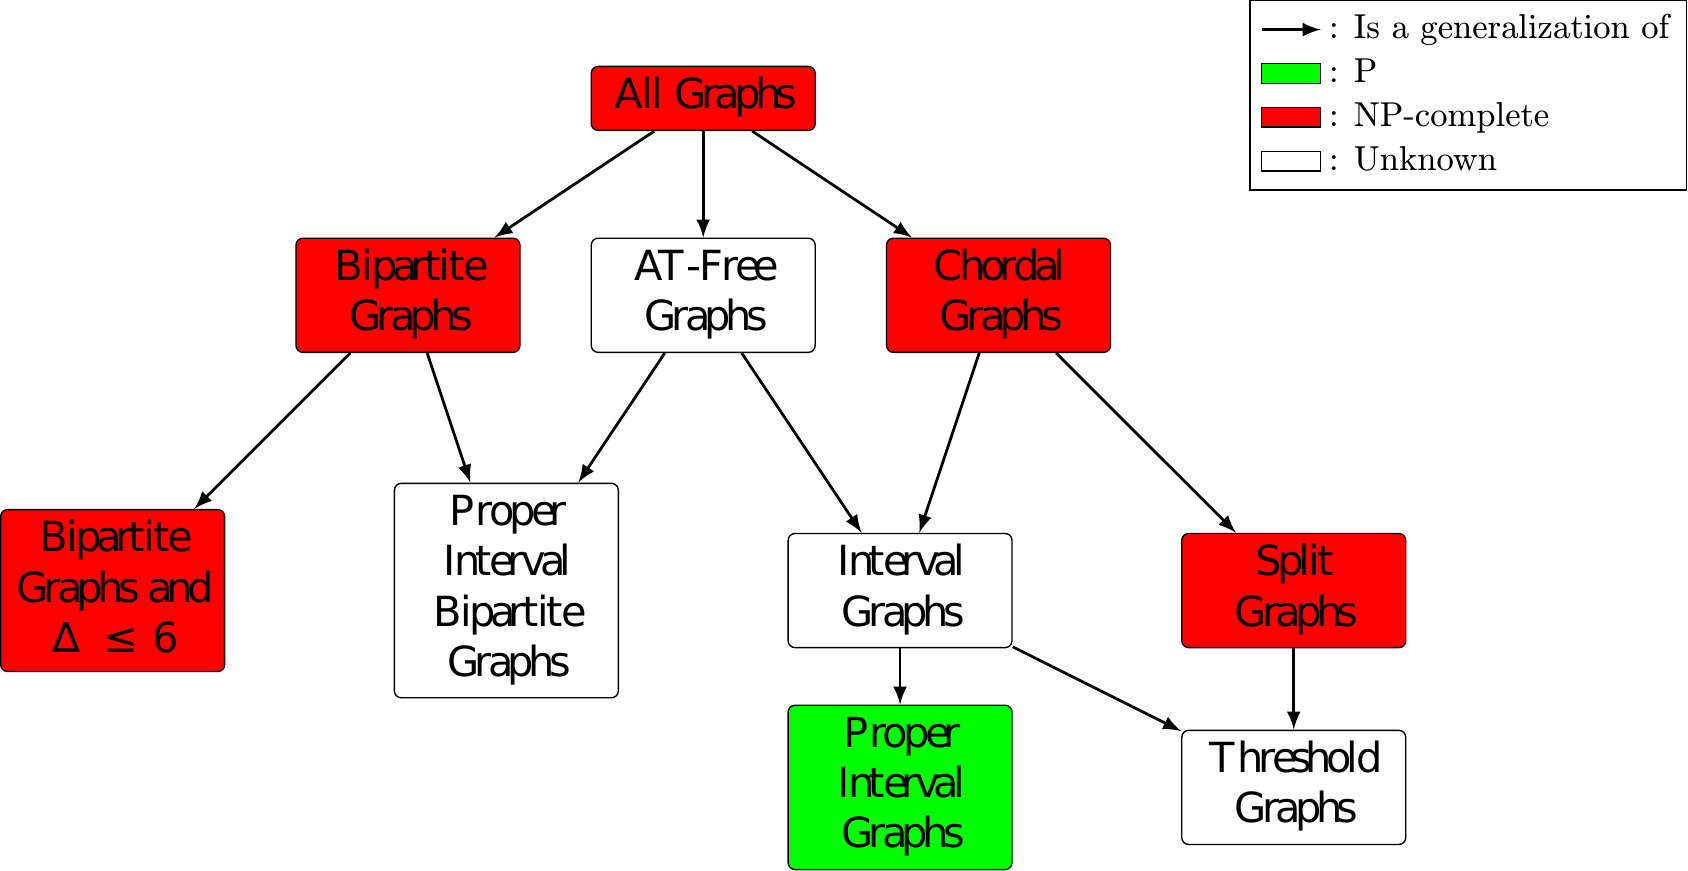}
	\caption{Overview complexity of the imbalance problem.}
\end{figure}
\subsection{Preliminaries}
\begin{figure}[H]
	\centering
	\input{figures/examplegraph.tex}
	\caption{Example graph $G=(V,E)$.}
	\label{ap-examplegraph}
	\input{figures/exampleordering.tex}
	\caption{Example ordering with imbalance $I(\sigma_V)= |2-0| + |2-1| + |1-2| + |0-1| + |0-1| = 6$.}
\end{figure}
\newpage
\begin{figure}[H]
	\centering
	\input{figures/examplerpibggraph.tex}
	\caption{Example of a restricted PI-bigraph $G=(X,Y,E)$, where $X$ is represented by the red vertices $x_i$ and $Y$ by the blue vertices $y_i$. The highlighted areas represent the vertex sets of $\mathscr{C}$.}
	\label{ap-rpibg}
	\input{figures/examplerpibg.tex}
	\caption{Interval representation of the restricted PI-bigraph of \cref{ap-rpibg}.}
	\label{ap-rpibg2}
\end{figure}
\subsection{Imbalance on Complete bipartite graphs}
\subsubsection{Proof of the upper bound}
$~$
\begin{figure}[H]
	\centering
	\input{figures/sandwichedexample.tex}
	\caption{Example of ``sandwiched'' ordering for $G = K_{4,9}$.}
	\label{ap-sandwichedexample}
	\input{figures/interwovenexample.tex}
	\caption{Example of ``interwoven'' ordering for $G = K_{3,9}$.}
	\label{ap-interwovenexample}
\end{figure}
\newpage
\subsubsection{Proof of the lower bound}
$~$
\begin{figure}[H]
	\centering
	\input{figures/k4-10.tex}
	\caption{Complete bigraph $G = K_{4,10}$.}
	\label{ap-k4-10}
	\input{figures/cbgdefsexample.tex}
	\caption{Visualization of the definitions of \cref{ap-compbigraphlower} with an ordering $\sigma_{X \cup Y}$ on the vertices of graph $G = K_{4,10}$.}
	\label{ap-cbgdefsexample}
		\begin{adjustbox}{max width=\textwidth}
			\begin{tabular}{ |c|c|c|c|c|c|c|c|c|c|c|c|c|c|c|c|c|c| }
				\hline
				& $L_0$ & $L_1$ & $L_2$ & $L_3$ & $\dots$ & $L_{k-3}$ & $L_{k-2}$ & $L_{k-1}$ & $L_{k}$ & $L_{k+1}$ & $L_{k+2}$ & $L_{k+3}$ & $\dots$ & $L_{|X|-3}$ & $L_{|X|-2}$ & $L_{|X|-1}$ & $L_{|X|}$ \\\hline
				
				$-S_0$ & $-$ & $+$ & $+$ & $+$ & $\dots$ & $+$ & $+$ & $+$ & $+$ & $+$ & $+$ & $+$ & $\dots$ & $+$ & $+$ & $+$ & $+$ \\ 
				$-S_1$ & $-$ & $-$ & $+$ & $+$ & $\dots$ & $+$ & $+$ & $+$ & $+$ & $+$ & $+$ & $+$ & $\dots$ & $+$ & $+$ & $+$ & $+$ \\ 
				$-S_2$ & $-$ & $-$ & $-$ & $+$ & $\dots$ & $+$ & $+$ & $+$ & $+$ & $+$ & $+$ & $+$ & $\dots$ & $+$ & $+$ & $+$ & $+$ \\
				
				$\vdots$ & $\vdots$ & $\vdots$ & $\vdots$ & $\ddots$ & $\vdots$ & $\vdots$ & $\vdots$ & $\vdots$ & $\vdots$ & $\vdots$ & $\vdots$ & $\vdots$ & $\ddots$ & $\vdots$ & $\vdots$ & $\vdots$ & $\vdots$ \\
				
				$-S_{k-2}$ & $-$ & $-$ & $-$ & $-$ & $\dots$ & $-$ & $-$ & $+$ & $+$ & $+$ & $+$ & $+$ & $\dots$ & $+$ & $+$ & $+$ & $+$ \\ 
				$-S_{k-1}$ & $-$ & $-$ & $-$ & $-$ & $\dots$ & $-$ & $-$ & $-$ & $+$ & $+$ & $+$ & $+$ & $\dots$ & $+$ & $+$ & $+$ & $+$ \\ 
				$S_k$ & $+$ & $+$ & $+$ & $+$ & $\dots$ & $+$ & $+$ & $+$ & $+$ & $-$ & $-$ & $-$ & $\dots$ & $-$ & $-$ & $-$ & $-$ \\
				$S_{k+1}$ & $+$ & $+$ & $+$ & $+$ & $\dots$ & $+$ & $+$ & $+$ & $+$ & $+$ & $-$ & $-$ & $\dots$ & $-$ & $-$ & $-$ & $-$ \\
				$S_{k+2}$ & $+$ & $+$ & $+$ & $+$ & $\dots$ & $+$ & $+$ & $+$ & $+$ & $+$ & $+$ & $-$ & $\dots$ & $-$ & $-$ & $-$ & $-$ \\
				
				$\vdots$ & $\vdots$ & $\vdots$ & $\vdots$ & $\ddots$ & $\vdots$ & $\vdots$ & $\vdots$ & $\vdots$ & $\vdots$ & $\vdots$ & $\vdots$ & $\vdots$ & $\ddots$ & $\vdots$ & $\vdots$ & $\vdots$ & $\vdots$ \\
				
				$S_{|X|-2}$ & $+$ & $+$ & $+$ & $+$ & $\dots$ & $+$ & $+$ & $+$ & $+$ & $+$ & $+$ & $+$ & $\dots$ & $+$ & $+$ & $-$ & $-$ \\
				$S_{|X|-1}$ & $+$ & $+$ & $+$ & $+$ & $\dots$ & $+$ & $+$ & $+$ & $+$ & $+$ & $+$ & $+$ & $\dots$ & $+$ & $+$ & $+$ & $-$ \\\hline
			\end{tabular}
		\end{adjustbox}
	$$(L_j, -S_i)=
	\begin{cases}
	- & \text{if } i \geq j \\
	+ & \text{if } i < j 
	\end{cases}
	$$
	$$(L_j, S_i)=
	\begin{cases}
	+ & \text{if } i \geq j \\
	- & \text{if } i < j 
	\end{cases}.$$
	\caption{Visualization of the table constructed in \cref{ap-lem2}.}
\end{figure}
\newpage
\subsection{Imbalance on Restricted Proper Interval bipartite graphs}
\begin{figure}[H]
	\centering
	\input{figures/examplerpibggraph2.tex}
	\caption{Illustration of the additional definitions of \cref{ap-c4} on the example graph of \cref{ap-rpibg}.}
	\label{ap-additionaldefsrpig}
\end{figure}
\subsubsection{Proof of the upper bound}
$~$
\begin{figure}[H]
	\centering
	\input{figures/ordconstrpibg1.tex}
	\caption{Example of an ordering where $s_{i-1}, s_{i} \in X_i$ and $G[C_i] = K_{6,6}$.}
	\input{figures/ordconstrpibg2.tex}
	\caption{Example of an ordering where $s_{i-1}\in X_i \wedge s_{i} \in Y_i$ and $G[C_i] = K_{6,6}$.}
\end{figure}
\newpage
\begin{figure}[H]
	\input{figures/ordconstrpibg3.tex}
	\caption{Example of an ordering  where $s_{i-1}, s_{i} \in X_i$ and $G[C_i] = K_{7,6}$.}
	\input{figures/ordconstrpibg4.tex}
	\caption{Example of an ordering  where $s_{i-1}, s_{i} \in Y_i$ and $G[C_i] = K_{7,6}$.}
	\input{figures/ordconstrpibg5.tex}
	\caption{Example of an ordering  where $s_{i-1} \in X_i \wedge s_{i} \in Y_i$ and $G[C_i] = K_{7,6}$.}
	\input{figures/k5-9.tex}
	\caption{Example complete bigraph $G = K_{5,9}$.}
	\label{ap-k5-9}
	\input{figures/oddoddcaseorderingsexample.tex}
	\caption{Suborderings corresponding to the graph in \cref{ap-k5-9}.}
	\label{ap-k5-9}
	\input{figures/ordconstrpibg6.tex}
	\caption{Example of an ordering  where $s_{i-1}, s_{i} \in Y_i$ and $G[C_i] = K_{5,9}$.}
\end{figure}
\newpage
\begin{figure}[H]
	\input{figures/ordconstrpibg7.tex}
	\caption{Example of an ordering  where $s_{i-1} \in Y_i \wedge s_{i} \in X_i$ and $G[C_i] = K_{5,9}$.}
	\input{figures/ordconstrpibg8.tex}
	\caption{Example of an ordering  where $s_{i-1} \in X_i \wedge s_{i} \in Y_i$ and $G[C_i] = K_{5,9}$.}
	\input{figures/ordconstrpibg9.tex}
	\caption{Example of an ordering  where $s_{i-1}, s_{i} \in X_i$ and $G[C_i] = K_{5,9}$.}
	\input{figures/largerpibgexample.tex}
	\caption{Example graph of \cref{ap-rpibg} with $s_0$ and $s_{n}$ assigned arbitrarily.}
	\input{figures/largerpibgorderingexample.tex}
	\caption{Suborderings $\sigma_{C_i}$ and the final constructed ordering $\sigma_{X\cup Y}$ of the graph in \cref{ap-orderingconstructionexample} created using the method.}
	\label{ap-orderingconstructionexample2}
\end{figure}
\newpage
\subsubsection{Proof of the lower bound}
$~$
\begin{figure}[H]
	\centering
	\input{figures/largerpibgexample2.tex}
	\caption{Illustration of $\mathscr{C} \setminus C_{k+1}$ and $C_{k+1}$.}
	\label{ap-largerpibgexample2}
\end{figure}

\section{Appendix - Full Proofs}
\subsection{Introduction}
Unfortunately, it is not possible to follow the same steps as the proof for the complexity result on proper interval graphs to prove linear time solvability on proper interval bipartite graphs. The proof for proper interval graphs uses the fact that a proper interval graph always has a special ordering called proper interval ordering, which is computable in linear time and yields minimum imbalance. We can find an analogous ordering for proper interval bipartite graphs by modifying the proof by Gardi \cite{GARDI20072906}. However, the analogous ordering does not always yield minimum imbalance.

\subsection{Preliminaries}

\subsection{Imbalance on Complete bipartite graphs}
\subsubsection{Proof of the upper bound}
$~$
\begin{case}
$(|X| \mod 2 = 1) \wedge (|Y| \mod 2 = 1).$\\
\begin{align*}
I(\sigma_{X \cup Y}) &= (|Y|-(|X|-1)+1)\cdot |X| + \Bigg(2\sum\limits_{i=1}^{(|X|-1)/2}|X|-2i\Bigg) \\
&+ \Bigg(2\sum\limits_{i=(|X|+1)/2}^{|X|-1}2i-|X|\Bigg) \\
&= (|Y|-|X|+2)\cdot |X| + \Bigg(2\sum\limits_{i=1}^{(|X|-1)/2}|X|-2i\Bigg) \\
&+ \Bigg(2\sum\limits_{i=1}^{(|X|-1)/2}2i +|X|-1-|X|\Bigg) \\
&= (|Y|-|X|+2)\cdot |X| + \Bigg(2\sum\limits_{i=1}^{(|X|-1)/2}|X|-2i\Bigg) \\
&+ \Bigg(2\sum\limits_{i=1}^{(|X|-1)/2}2i-1\Bigg) \\
&= (|Y|-|X|+2)\cdot |X| + \Bigg(2\sum\limits_{i=1}^{(|X|-1)/2}|X|-1\Bigg) \\
&= (|Y|-|X|+2)\cdot |X| + \Big((|X|-1)\cdot|X|-(|X|-1)\Big) \\
&= |Y|\cdot|X| -|X|^2+2|X| + |X|^2-|X|-|X|+1 \\
&= |Y|\cdot|X|+1\\
&= |X|\cdot |Y| + (|X| \mod 2) \cdot (|Y| \mod 2).
\end{align*}
\end{case}

\subsubsection{Proof of the lower bound}
\begin{lemma}\label{ap-lmacbg2}
	If $G = (X,Y,E)$ is a complete bigraph, then 
	$$I(G) \geq |X|\cdot |Y| + (|X| \mod 2) \cdot (|Y| \mod 2).$$
\end{lemma}
\begin{proof}
	We shall prove the lemma by showing that for any case $k$, where $0 \leq k \leq |X| + 1$, and arbitrary ordering $\sigma_{X\cup Y}$, $I(\sigma_{X \cup Y})$ is bounded from below by $|X|\cdot |Y| + (|X| \mod 2) \cdot (|Y| \mod 2)$.\\
	\begin{align}
	I(\sigma_{X \cup Y}) &= \Bigg(\sum\limits_{i=0}^{|X|}L_i \cdot ||X|-2i|\Bigg) + \sum\limits_{i=0}^{|X|-1}|S_i| \notag  \\
	&= \Bigg(\sum\limits_{i=0}^{\lfloor|X|/2\rfloor}L_i \cdot (|X|-2i)\Bigg) + \Bigg(\sum\limits_{i=\lfloor|X|/2\rfloor+1}^{|X|}L_i \cdot (2i-|X|)\Bigg)\notag  \\ 
	&+ \Bigg(\sum\limits_{i=k}^{|X|-1}S_i\Bigg) - \Bigg(\sum\limits_{i=0}^{k-1}S_i\Bigg) \notag  \\
	&= \Bigg(\sum\limits_{i=0}^{\lfloor|X|/2\rfloor}L_i \cdot (|X|-2i|)\Bigg) + \Bigg(\sum\limits_{i=\lfloor|X|/2\rfloor+1}^{|X|}L_i \cdot (2i-|X|)\Bigg) \notag\\ 
	&+ \Bigg(\sum\limits_{i=0}^{k}(|X|-2k+2i)\cdot L_i\Bigg) + \Bigg(\sum\limits_{i=k+1}^{|X|}(|X|+2k-2i)\cdot L_i\Bigg), \label{ap-eqlem3-1}
	\end{align}
	where \cref{ap-eqlem3-1} follows from \cref{lem2}.
	
	\begin{case}\label{ap-cbgc31}
		$|X| \mod 2 = 0$.\\
		Consider case $k$, where $k < |X|/2$. We have $S_k \geq 0$ if and only if 
		\begin{align}
		\sum\limits_{j=0}^{k}L_j \geq \sum\limits_{j=k+1}^{|X|}L_j. \label{ap-eqlem3-2}
		\end{align}
		From \cref{ap-eqlem3-1} we have:
		\begin{align}
		I(\sigma_{X \cup Y}) &= \Bigg(\sum\limits_{i=0}^{k}(|X|-2i)\cdot L_i\Bigg) + \Bigg(\sum\limits_{i=k+1}^{|X|/2}(|X|-2i) \cdot L_i\Bigg) \notag\\
		&+ \Bigg(\sum\limits_{i=|X|/2+1}^{|X|}(2i-|x|) \cdot L_i\Bigg) \notag + \Bigg(\sum\limits_{i=0}^{k}(|X|-2k+2i)\cdot L_i\Bigg) \notag\\ 
		&+ \Bigg(\sum\limits_{i=k+1}^{|X|/2}(|X|+2k-2i) \cdot L_i\Bigg) + \Bigg(\sum\limits_{i=|X|/2+1}^{|X|}(|X|+2k-2i) \cdot L_i\Bigg) \label{ap-eqlem3-2.5}\\
		&= \Bigg(\sum\limits_{i=0}^{k}(2|X|-2k)\cdot L_i\Bigg) + \Bigg(\sum\limits_{i=k+1}^{|X|/2}(2|X|+2k-4i) \cdot L_i\Bigg) \notag\\ 
		&+ \Bigg(\sum\limits_{i=|X|/2+1}^{|X|}2k \cdot L_i\Bigg) \notag\\
		&= \Bigg(\sum\limits_{i=0}^{k}|X| \cdot L_i\Bigg) + 
		\Bigg(\sum\limits_{i=0}^{k}(|X|-2k)\cdot L_i\Bigg) \notag \\ 
		&+ \Bigg(\sum\limits_{i=k+1}^{|X|/2}(2|X|+2k-4i) \cdot L_i\Bigg) + \Bigg(\sum\limits_{i=|X|/2+1}^{|X|}2k \cdot L_i\Bigg) \notag\\
		&\geq \Bigg(\sum\limits_{i=0}^{k}|X| \cdot L_i\Bigg) + 
		\Bigg(\sum\limits_{i=k+1}^{|X|}(|X|-2k)\cdot L_i\Bigg)\notag  \\ 
		&+ \Bigg(\sum\limits_{i=k+1}^{|X|/2}(2|X|+2k-4i) \cdot L_i\Bigg) + \Bigg(\sum\limits_{i=|X|/2+1}^{|X|}2k \cdot L_i\Bigg) \label{ap-eqlem3-3}\\
		&= \Bigg(\sum\limits_{i=0}^{k}|X| \cdot L_i\Bigg) + \Bigg(\sum\limits_{i=k+1}^{|X|/2}(3|X|-4i) \cdot L_i\Bigg) + \Bigg(\sum\limits_{i=|X|/2+1}^{|X|}|X| \cdot L_i\Bigg) \notag\\
		&\geq \Bigg(\sum\limits_{i=0}^{k}|X| \cdot L_i\Bigg) + \Bigg(\sum\limits_{i=k+1}^{|X|/2}|X| \cdot L_i\Bigg) + \Bigg(\sum\limits_{i=|X|/2+1}^{|X|}|X| \cdot L_i\Bigg) \label{ap-eqlem3-4}\\
		&= |X| \cdot \sum\limits_{i=0}^{|X|}L_i \notag \\
		&= |X|\cdot|Y|, \notag
		\end{align} %TODO
		where \cref{ap-eqlem3-2.5} and \cref{ap-eqlem3-4} follows from the assumption that $k < |X|/2$, and \cref{ap-eqlem3-3} follows from \cref{ap-eqlem3-2}.
		
		Consider case $k$, where $k = |X|/2$. From \cref{ap-eqlem3-1} and the assumption that $k = |X|/2$ we have:
		\begin{align*}
		I(\sigma_{X \cup Y}) &= \Bigg(\sum\limits_{i=0}^{|X|/2}L_i \cdot (|X|-2i|)\Bigg) + \Bigg(\sum\limits_{i=|X|/2+1}^{|X|}L_i \cdot (2i-|X|)\Bigg)  \notag\\ 
		&+ \Bigg(\sum\limits_{i=0}^{|X|/2}(|X|-2|X|/2+2i)\cdot L_i\Bigg) \\
		&+ \Bigg(\sum\limits_{i=|X|/2+1}^{|X|}(|X|+2|X|/2-2i)\cdot L_i\Bigg) \\
		&= \Bigg(\sum\limits_{i=0}^{|X|/2}L_i \cdot |X|\Bigg) + \Bigg(\sum\limits_{i=|X|/2+1}^{|X|}L_i \cdot |X|\Bigg)\\
		&= |X| \cdot \sum\limits_{i=0}^{|X|}L_i \\
		&= |X| \cdot |Y|.
		\end{align*}
		Consider case $k$, where $k > |X|/2$. We have $S_{k-1} < 0$ if and only if
		\begin{align}
		\sum\limits_{j=0}^{k-1}L_j < \sum\limits_{j=k}^{|X|}L_j. \label{ap-eqlem3-5}
		\end{align}
		From \cref{ap-eqlem3-1} we have:
		\begin{align}
		I(\sigma_{X \cup Y}) &= \Bigg(\sum\limits_{i=0}^{|X|/2}(|X|-2i|) \cdot L_i\Bigg) + \Bigg(\sum\limits_{i=|X|/2+1}^{k}(2i-|X|)\cdot L_i\Bigg) \notag\\
		&+ \Bigg(\sum\limits_{i=k+1}^{|X|}(2i-|X|)\cdot L_i\Bigg) \notag + \Bigg(\sum\limits_{i=0}^{|X|/2}(|X|-2k+2i) \cdot L_i\Bigg) \notag\\ 
		&+ \Bigg(\sum\limits_{i=|X|/2+1}^{k}(|X|-2k+2i) \cdot L_i\Bigg) + \Bigg(\sum\limits_{i=k+1}^{|X|}(|X|+2k-2i) \cdot L_i\Bigg) \label{ap-eqlem3-5.5} \\
		&= \Bigg(\sum\limits_{i=0}^{|X|/2}L_i \cdot (2|X|-2k)\Bigg) + \Bigg(\sum\limits_{i=|X|/2+1}^{k}(4i-2k)\cdot L_i\Bigg) \notag\\
		&+ \Bigg(\sum\limits_{i=k+1}^{|X|}2k\cdot L_i\Bigg) \notag \\
		&= \Bigg(\sum\limits_{i=0}^{|X|/2}L_i \cdot (2|X|-2k)\Bigg) + \Bigg(\sum\limits_{i=|X|/2+1}^{k-1}(4i-2k)\cdot L_i\Bigg) \notag\\
		&+ \Bigg(\sum\limits_{i=k}^{|X|}2k\cdot L_i\Bigg) \notag \\
		&= \Bigg(\sum\limits_{i=0}^{|X|/2}L_i \cdot (2|X|-2k)\Bigg) + \Bigg(\sum\limits_{i=|X|/2+1}^{k-1}(4i-2k)\cdot L_i\Bigg) \notag \\ 
		&+ \Bigg(\sum\limits_{i=k}^{|X|}|X|\cdot L_i\Bigg) + \Bigg(\sum\limits_{i=k}^{|X|}(2k-|X|)\cdot L_i\Bigg) \notag\\
		&> \Bigg(\sum\limits_{i=0}^{|X|/2}L_i \cdot (2|X|-2k)\Bigg) + \Bigg(\sum\limits_{i=|X|/2+1}^{k-1}(4i-2k)\cdot L_i\Bigg) \notag\\ 
		&+ \Bigg(\sum\limits_{i=k}^{|X|}|X|\cdot L_i\Bigg) + \Bigg(\sum\limits_{i=0}^{k-1}(2k-|X|)\cdot L_i\Bigg) \label{ap-eqlem3-6}\\
		&= \Bigg(\sum\limits_{i=0}^{|X|/2}L_i \cdot |X|\Bigg) + \Bigg(\sum\limits_{i=|X|/2+1}^{k-1}(4i-|X|)\cdot L_i\Bigg) + \Bigg(\sum\limits_{i=k}^{|X|}|X|\cdot L_i\Bigg) \notag \\
		&\geq \Bigg(\sum\limits_{i=0}^{|X|/2}L_i \cdot |X|\Bigg) + \Bigg(\sum\limits_{i=|X|/2+1}^{k-1}(|X|+4)\cdot L_i\Bigg) + \Bigg(\sum\limits_{i=k}^{|X|}|X|\cdot L_i\Bigg) \label{ap-eqlem3-7}\\
		&\geq |X| \cdot \sum\limits_{i=0}^{|X|}L_i \notag\\
		&= |X| \cdot |Y|, \notag
		\end{align}
		where \cref{ap-eqlem3-5.5} and \cref{ap-eqlem3-7} follows from the assumption that $k > |X|/2$, and \cref{ap-eqlem3-6} follows from \cref{ap-eqlem3-5}.
	\end{case}
	\begin{case}
		$|X| \mod 2 = 1$.\\
		For $\oplus \in \{<, =, >\}$, let case $k \oplus |X|/2$ be the abbreviation of case $k$, where $k \oplus |X|/2$.
		
		Since $|X|$ is odd, the case $k = |X|/2$ does not exist as $k \in \mathbb{N}$. Thus we only need to consider case $k < |X|/2$ and case $k > |X|/2$. The analysis for these cases are the same as the analysis for case $k < |X|/2$ and case $k > |X|/2$ in \cref{ap-cbgc31}.
		
		If $|Y| \mod 2 = 1$, then $S_i \neq 0$ for all $0 \leq i \leq |X|-1$, since it is impossible to partition $Y$ such that 
		$$\sum\limits_{j=0}^{i}L_j = \sum\limits_{j=i+1}^{|X|}L_j.$$
		Thus for the analysis of case $k < |X|/2$, we have $S_k \geq 0$ if and only if
		$$\sum\limits_{j=0}^{i}L_j > \sum\limits_{j=i+1}^{|X|}L_j.$$
		Instead of the non-strict inequality in \cref{ap-eqlem3-2}, we have a strict inequality. Therefore, when applying \cref{ap-eqlem3-2} for the derivation step at \cref{ap-eqlem3-3}, we have a strict inequality. Thus, when $|Y|$ is odd, in both case $k < |X|/2$ and $k > |X|/2$ we have 
		$$I(\sigma_{X\cup Y}) > |X| \cdot |Y|.$$
	\end{case}
\end{proof}

\subsection{Imbalance on Restricted Proper Interval bipartite graphs}

\subsubsection{Proof of the upper bound}

\begin{lemma}
	Let $G = (X,Y,E)$ be a restricted PI-bigraph with corresponding family of maximal subsets $\mathscr{C} = \{C_1, \dots, C_n\}$. Let $C_i \in \mathscr{C}$ such that $|X_i| = 1$ or $|Y_i| = 1$. W.l.o.g. assume that $|X_i| = 1$, then neither overlapping vertices $s_{i-1}$ nor $s_i$ can be in $X_i$. Formally, for all $C_i \in \mathscr{C}$,
	$$|X_i| = 1 \implies s_{i-1} \notin X_i \wedge s_{i} \notin X_i$$ 
	and
	$$|Y_i| = 1 \implies s_{i-1} \notin Y_i \wedge s_{i} \notin Y_i.$$ 
\end{lemma}
\begin{proof}
	Assume that a vertex set $C_i \in \mathscr{C}$ exists such that 
	$$\big(|X_i| = 1 \wedge (s_{i-1} \in X_i \vee s_{i} \in X_i)\big) \vee \big(|Y_i| = 1 \wedge (s_{i-1} \in Y_i \vee s_{i} \in Y_i)\big).$$ 
	W.l.o.g. assume that $|X_i| = 1 \wedge s_{i} \in X_i$. Then $G[C_i \cup Y_{i+1}]$ is a complete bigraph. This contradicts the maximality of $C_i$. Thus, there exists no $C_i \in \mathscr{C}$ such that 
	$$\big(|X_i| = 1 \wedge (s_{i-1} \in X_i \vee s_{i} \in X_i)\big) \vee \big(|Y_i| = 1 \wedge (s_{i-1} \in Y_i \vee s_{i} \in Y_i)\big).$$
\end{proof}

\subsubsection{Proof of the lower bound}
