# Supplementary material for: Characterization of the Imbalance Problem on Complete Bipartite Graphs
Source: arXiv:2111.00154 source file (2021-11-20)
Supplement: Supplementary file 2 [file appendix-figures.tex]

\section{Appendix - Figures}
\setcounter{subsection}{3}
\subsection{Imbalance on Restricted Proper Interval bipartite graphs}
\subsubsection{Proof of the lower bound}
